# Supplementary material for: Optomechanical self-organization in a mesoscopic atom array
Source: arXiv:2410.12754 source file (2025-05-26)
Supplement: Supplementary file 1 [file Optomechanical_Dicke_nphys_SI_20250402.pdf]

# Supplementary Information

## I. THEORETICAL MODEL

The theoretical prediction of the critical drive strength is derived from an effective two dimensional model where the atoms move along and perpendicular to the cavity axis ($z$-axis). Of the two directions perpendicular to the cavity axis, we consider the one ($x$-axis) along the direction of the pump. Motional effects along the remaining direction can be neglected as the beam waist of the pump is much larger than the spread of the atomic wavefunction. Each tweezer trap is approximated by a harmonic potential, and the atoms are assumed to be two-level systems of mass $M$. The degrees of freedom of the system are thus the internal ground $|g\rangle$ and excited $|e\rangle$ states of the atoms, the position $\hat{z}_j, \hat{x}_j$ and momentum $\hat{p}_{zj}, \hat{p}_{xj}$ operators of each atom, and the cavity field described by the bosonic creation $\hat{c}^\dagger$ and annihilation $\hat{c}$ operators for a photon in the cavity. The dynamics of the system obeys the master equation

$$\dot{\hat{\rho}}_{\rm tot} = -\frac{\rm i}{\hbar}[\hat{H}_{\rm tot}, \hat{\rho}_{\rm tot}] + \kappa\left(2\hat{c}\hat{\rho}_{\rm tot}\hat{c}^\dagger - \left\{\hat{c}^\dagger\hat{c}, \hat{\rho}_{\rm tot}\right\}\right) + \gamma\sum_j\left(2\int {\rm d}\mathbf{n}\,\mathcal{N}(\mathbf{n})\,e^{-{\rm i}k_0\mathbf{n}\cdot\hat{\mathbf{r}}_j}\hat{\sigma}_j^-\hat{\rho}_{\rm tot}e^{{\rm i}k_0\mathbf{n}\cdot\hat{\mathbf{r}}_j}\hat{\sigma}_j^+ - \left\{\hat{\sigma}_j^+\hat{\sigma}_j^-, \hat{\rho}_{\rm tot}\right\}\right), \tag{S1}$$

where $\hat{\sigma}_j^+ \equiv |e_j\rangle\langle g_j| = (\hat{\sigma}_j^-)^\dagger$ are the atomic coherence operators. The second term in Eq. (S1) describes the decay of the cavity field, where $\kappa$ is the cavity half-linewidth. The last term describes the atomic decay into free space including recoil effects. Here, $k_0 = \omega_a/c$, $\gamma$ is the atomic half-linewidth, $\mathcal{N}(\mathbf{n})$ is the dipole emission pattern, and the integral is taken over all directions in space represented by the unit vector $\mathbf{n}$. We define the position operator for the atom $j$ in the $xz$-plane as $\hat{\mathbf{r}}_j = (\hat{x}_j, \hat{z}_j)$. The Hamiltonian that describes the coupling between the atoms and the cavity, written in the frame rotating at the frequency of the pump $\omega_{\rm p}$, reads

$$\hat{H}_{\rm tot} \equiv \sum_{j=1}^{N}\left\{\frac{\hat{\mathbf{p}}_j^2}{2M} + \frac{M\nu^2}{2}\left[(\hat{z}_j - z_{0j})^2 + \hat{x}_j^2\right] - \hbar\Delta_{\rm pa}\hat{\sigma}_j^+\hat{\sigma}_j^- + \frac{\hbar\Omega(\hat{x}_j)}{2}(\hat{\sigma}_j^+ + \hat{\sigma}_j^-) + \hbar g_0\sin(k\hat{z}_j)\left(\hat{c}^\dagger\hat{\sigma}_j^- + \hat{\sigma}_j^+\hat{c}\right)\right\} - \hbar\Delta_{\rm pc}\hat{c}^\dagger\hat{c}. \tag{S2}$$

Here, $\Delta_{\rm pc} \equiv \omega_{\rm p} - \omega_{\rm c}$ and $\Delta_{\rm pa} \equiv \omega_{\rm p} - \omega_{\rm a}$ are the pump detunings from the cavity frequency ($\omega_{\rm c}$) and atomic frequency ($\omega_{\rm a}$) respectively, and $\nu$ is the trap frequency of the tweezers. We assume the foci of the tweezers lie parallel to the cavity axis, where $z_{0j}$ is the position of the tweezer trap for the $j$-th atom. We approximate the spatial profile of the cavity field as $\sin(kz)$, with wave vector $k = 2\pi/\lambda$. The side pump driving the atoms consists of two counter propagating beams, which result in a standing wave profile $\Omega(x) = \Omega\cos(k_p x)$ whose maximum is located at the position of the atoms. Here, $k_p \simeq k$ is the pump wave-vector. We assume the atoms to be driven in phase, which is achieved by aligning the atomic array orthogonal to the pump direction.

The experiment is operated in the limit of large pump-atom detuning, $\Delta_{\rm pa} \gg \{g_0, \Omega, \kappa, \gamma\}$. Hence, we adiabatically eliminate the internal atomic degrees of freedom assuming linear response (that is $\langle\hat{\sigma}_j^z\rangle \simeq -1$) and neglecting atomic free-space decay. Within this approximation, the dynamics of the system obeys the effective master equation

$$\partial_t\hat{\rho}_{\rm om} = -\frac{\rm i}{\hbar}\left[\hat{H}_{\rm om}, \hat{\rho}\right] + \kappa\left(2\hat{c}\hat{\rho}_{\rm om}\hat{c}^\dagger - \left\{\hat{c}^\dagger\hat{c}, \hat{\rho}_{\rm om}\right\}\right), \tag{S3}$$

where $\hat{\rho}_{\rm om}$ describes the state of the atomic motion and of the cavity field. The second term in Eq. (S3) represents the damping of the cavity, and the effective optomechanical Hamiltonian that describes the coupling of the atomic motion to the cavity field reads

$$\begin{aligned}\hat{H}_{\rm om} =& \sum_{j=1}^{N}\left\{\frac{\hat{\mathbf{p}}_j^2}{2M} + \frac{M}{2}\nu^2\left[\hat{x}_j^2 + (\hat{z}_j - z_{0j})^2\right] - \frac{\hbar\Omega^2}{4\Delta_{\rm pa}}\cos^2(k\hat{x}_j)\right\} - \hbar\Delta_{\rm pc}\hat{c}^\dagger\hat{c} \\ &+ \frac{\hbar g_0}{2\Delta_{\rm pa}}\left(\hat{c}^\dagger + \hat{c}\right)\sum_{j=1}^{N}\Omega(\hat{x}_j)\sin(k\hat{z}_j) + \frac{\hbar g_0^2}{\Delta_{\rm pa}}\hat{c}^\dagger\hat{c}\sum_{j=1}^{N}\sin^2(k\hat{z}_j),\end{aligned} \tag{S4}$$

The optomechanical coupling is described by the first and second terms in the second line of Eq. (S4). The latter is the well-known coupling arising from radiation pressure forces and is common to several optomechanical systems [S1]. It describes the dispersive shift of the cavity frequency due to the atoms and the back-action of the cavity on the atomic trap frequency (known as the "optical spring effect"). The former, instead, arises from the coherent scattering

of photons from the pump into the cavity and so depends on the Rabi frequency of the pump [S2–S4]. This term produces a force proportional to the cavity field that shifts the atomic equilibrium position away from the nodes. These two coupling terms can be tuned independently. In particular, by changing the Rabi frequency of the pump $\Omega$ while keeping the ratio $g_0/\Delta_{\rm pa}$ fixed, one can make the coherent scattering dominate over the radiation pressure coupling.

We remark that a very similar model has been considered for driven atomic clouds in optical cavities, considered for instance in Refs. [S5–S8]. The difference here is given by the tweezer traps, which add an additional time-scale of the order $1/\nu$ for the motional dynamics of the atoms. As we will see below, this leads to a change in the critical pump strength ($\Omega_{\rm c}$) responsible for atomic self-organization. This model is justified for values of $\Omega$ below and around the transition point where atomic saturation is negligible. Above the transition ($\Omega > \Omega_{\rm c}$), the buildup of the cavity field leads to non-negligible saturation of the atoms, and to diffusion of the internal excitation to other internal levels. This latter effect leads to the breakdown of the two-level approximation for the atoms. However, the model is sufficient for the purpose of deriving the value of the critical pump strength $\Omega_{\rm c}$ as we now discuss.

## II. DERIVATION OF THE CRITICAL PUMP STRENGTH $\Omega_{\rm c}$

In the absence of the pump ($\Omega = 0$) and with tweezers placed at the cavity field nodes, i.e. $z_{0j} = jn\lambda$ for any integer or half integer $n$, the steady state solution of Eq. (S3) corresponds to the cavity in vacuum and the atoms in the thermal state of the harmonic tweezers potential. As $\Omega$ is increased, the atoms start to scatter photons into the cavity, which act back on the atoms modifying the effective trap frequency. At the critical value $\Omega_{\rm c}$, the solution of atoms at the nodes becomes unstable, leading to self-organization towards the cavity antinodes for $\Omega > \Omega_{\rm c}$. To compute $\Omega_{\rm c}$, we take a mean field approach where correlations between the cavity and the atomic motion are neglected [S9]. It is instructive to first consider the case where atoms are allowed to move only along the cavity axis. In the following we thus consider an effective one-dimensional model for the atomic motion. We will later generalize the results to two dimensions.

### A. 1D Motion

The effective optomechanical model for atoms moving along the cavity axis only is obtained from Eq. (S3) assuming $\Omega(x) = \Omega$ in Eq. (S4). According to the mean field approximation, we consider the system dynamics to be confined to the product state manifold defined by

$$\hat{\rho}_{\rm MF} = |\alpha\rangle\langle\alpha| \otimes \hat{\rho}_{\rm at}, \tag{S5}$$

where $\hat{\rho}_{\rm at}$ is the density matrix of the atomic motion, and $|\alpha\rangle$ the coherent state of the cavity field. In this case, the evolution of the atomic motional state reads

$$\dot{\hat{\rho}}_{\rm at} = -\frac{\rm i}{\hbar}[\hat{H}_{\rm 1D}, \hat{\rho}_{\rm at}] - {\rm i}\frac{\Omega g_0}{2\Delta_{\rm pa}}(\alpha + \alpha^*)\left[\sum_{j=1}^{N}\sin(k\hat{z}_j), \hat{\rho}_{\rm at}\right] - {\rm i}|\alpha|^2\frac{g_0^2}{\Delta_{\rm pa}}\left[\sum_{j=1}^{N}\sin^2(k\hat{z}), \hat{\rho}_{\rm at}\right], \tag{S6}$$

where we defined the field amplitude $\alpha \equiv \langle\hat{c}\rangle$, and the Hamiltonian $\hat{H}_{\rm 1D} \equiv \sum_j \left[\hat{p}_j^2/2M + M\nu^2(\hat{z}_j - z_{0j})^2/2\right]$. The evolution of the average cavity field $\alpha$ depends on the mean field dynamics of the $N$ atoms and reads

$$\dot{\alpha} = \left[{\rm i}\left(\Delta_{\rm pc} - \frac{g_0^2}{\Delta_{\rm pa}}\sum_{j=1}^{N}\langle\sin^2(k\hat{z}_j)\rangle\right) - \kappa\right]\alpha - {\rm i}\frac{g_0\Omega}{2\Delta_{\rm pa}}\left\langle\sum_{j=1}^{N}\sin(k\hat{z}_j)\right\rangle, \tag{S7}$$

where $\langle\cdot\rangle = {\rm Tr}[\cdot\hat{\rho}_{\rm at}]$. We proceed to linearize the system around the solution in Eq. (S5) with $\alpha = 0$ and where each atom is in the thermal state $\hat{\rho}_{\rm th} \equiv \exp(-\beta\hat{H}_{\rm 1D})/\mathcal{Z}$, with $\beta = 1/k_BT$ and $\mathcal{Z} \equiv {\rm Tr}[\exp(-\beta\hat{H}_{\rm 1D})]$. Accordingly, we make the substitution $\alpha \to \delta\alpha$ and $\hat{\rho}_{\rm at} \to \hat{\rho}_{\rm th} + \delta\hat{\rho}$ in Eqs. (S6) and (S7), and keep only terms linear in the fluctuations. We readily find

$$\begin{aligned}\delta\dot{\hat{\rho}} =& \mathcal{L}_0\delta\hat{\rho} - {\rm i}\frac{\Omega g_0}{2\Delta_{\rm pa}}(\delta\alpha + \delta\alpha^*)\Big[\sum_{j=1}^{N}\sin(k\hat{z}_j), \hat{\rho}_{\rm th}\Big],\\ \delta\dot{\alpha} =& \Big[{\rm i}\Big(\Delta_{\rm pc} - \frac{g_0^2}{\Delta_{\rm pa}}\sum_{j=1}^{N}\langle\sin^2(k\hat{z}_j)\rangle_{\rm th}\Big) - \kappa\Big]\delta\alpha - {\rm i}\frac{g_0\Omega}{2\Delta_{\rm pa}}{\rm Tr}\Big[\sum_{j=1}^{N}\sin(k\hat{z}_j)\delta\hat{\rho}\Big].\end{aligned} \tag{S8}$$

Here, we defined the superoperator $\mathcal{L}_0\hat{\rho} \equiv -\mathrm{i}\hbar^{-1}[\hat{H}_{1\mathrm{D}}, \hat{\rho}]$, and $\langle\cdot\rangle_{\mathrm{th}} \equiv \mathrm{Tr}[\cdot\hat{\rho}_{\mathrm{th}}]$ for convenience of notation.

The critical pump strength $\Omega_{\mathrm{c}}$ corresponds to the pole of the susceptibility of the system [S9, S10]. To compute the susceptibility, we take the Laplace transform of Eq. (S8). We define $\tilde{\hat{\rho}} = \int_0^\infty \mathrm{d}t\, e^{-st}\delta\hat{\rho}(t)$ and $\tilde{\alpha} = \int_0^\infty \mathrm{d}t\, e^{-st}\delta\alpha(t)$, where $s = -\mathrm{i}\omega + \epsilon$, with $\epsilon > 0$ to ensure the analyticity of the susceptibility in the upper-half complex plane [S10]. The Laplace transform of the atomic operator reads

$$\tilde{\hat{\rho}} = (s\mathbb{I} - \mathcal{L}_0)^{-1}\,\delta\hat{\rho}(0) - \mathrm{i}\frac{g_0\Omega}{2\Delta_{\mathrm{pa}}}\,(\tilde{\alpha} + \tilde{\alpha}^*)\,(s\mathbb{I} - \mathcal{L}_0)^{-1}\left[\sum_{j=1}^{N}\sin(k\hat{z}_j), \hat{\rho}_{\mathrm{th}}\right], \tag{S9}$$

where $\mathbb{I}$ is the identity superoperator, and $\delta\hat{\rho}(0)$ is the initial condition of the linear fluctuation of the atomic density operator. Substituting Eq. (S9) into the equation for the cavity field we obtain the solution

$$\mathcal{A}(s)\tilde{\alpha} + \mathcal{C}(s)\tilde{\alpha}^* = \alpha(0) - \mathrm{i}\frac{g_0\Omega}{2\Delta_{\mathrm{pa}}}N\mathrm{Tr}\left\{\sum_{j=1}^{N}\sin(k\hat{z}_j)\,(s - \mathcal{L}_0)^{-1}\,\delta\hat{\rho}(0)\right\}, \tag{S10}$$

where $\alpha(0)$ is the initial condition for the cavity field fluctuations and we have defined

$$\mathcal{A}(s) \equiv s - \mathrm{i}\Big(\Delta_{\mathrm{pc}} - \frac{g_0^2}{\Delta_{\mathrm{pa}}}\sum_{j=1}^{N}\left\langle\sin^2(k\hat{z}_j)\right\rangle_{\mathrm{th}}\Big) + \kappa + \mathcal{C}(s), \tag{S11}$$

and

$$\begin{aligned}\mathcal{C}(s) &= \left(\frac{g_0\Omega N}{2\Delta_{\mathrm{pa}}}\right)^2\mathrm{Tr}\left\{\hat{\Theta}(s\mathbb{I} - \mathcal{L}_0)^{-1}\left[\hat{\Theta}, \hat{\rho}_{\mathrm{th}}\right]\right\} = \left(\frac{g_0\Omega N}{2\Delta_{\mathrm{pa}}}\right)^2\int_0^\infty \mathrm{d}t\, e^{-st}\,\mathrm{Tr}\left\{\hat{\Theta}e^{\mathcal{L}_0 t}\left[\hat{\Theta}, \hat{\rho}_{\mathrm{th}}\right]\right\} \\ &= \left(\frac{g_0\Omega N}{2\Delta_{\mathrm{pa}}}\right)^2\int_0^\infty \mathrm{d}t\, e^{-st}\left\langle\left[\hat{\Theta}(t), \hat{\Theta}\right]\right\rangle_{\mathrm{th}},\end{aligned} \tag{S12}$$

where we defined the operator

$$\hat{\Theta} \equiv \frac{1}{N}\sum_{j=1}^{N}\sin(k\hat{z}_j). \tag{S13}$$

In Eq. (S12), we employed the Laplace transform identity $(s\mathbb{I} - \mathcal{L}_0)^{-1} = \int_0^\infty \mathrm{d}t\, e^{-(s\mathbb{I} - \mathcal{L}_0)t}$ in the first passage. From the first to the second line, we used the adjoint action of the operator $\exp(\mathcal{L}_0 t)$ to transform the Schrödinger operator $\hat{\Theta}$ into the Heisenberg operator $\hat{\Theta}(t)$. Note that $\hat{\Theta} = \hat{\Theta}(0)$.

These equations have a simple physical interpretation. The correlator appearing in Eq. (S12) corresponds to the linear response function of the operator $\hat{\Theta}$ [S10] that defines the mechanical response to the force exerted by the scattering of photons into the cavity. From Eq.(S11), we interpret $\mathcal{C}(s)$ as the effective shift to the cavity response due to the backaction of the atoms on the cavity field arising from coherent scattering. The appearance of the operator $\hat{\Theta}$ indicates that this shift depends on the collective self-organization of the atoms. Additionally, the non-linear dependence on $\hat{z}$ accounts for the non-linear correction to the mechanical response of the system as we shall see below.

The dynamics of the cavity field is thus found by solving the following system of equations and taking the inverse Laplace transform

$$R(s)\begin{pmatrix}\tilde{\alpha} \\ \tilde{\alpha}^*\end{pmatrix} = \begin{pmatrix}\alpha(0) - \mathrm{i}\frac{g_0\Omega}{2\Delta_{\mathrm{pa}}}\mathrm{Tr}\left[\hat{\Theta}\,(s\mathbb{I} - \mathcal{L}_0)^{-1}\,\delta\hat{\rho}(0)\right] \\ \alpha^*(0) + \mathrm{i}\frac{g_0\Omega}{2\Delta_{\mathrm{pa}}}\mathrm{Tr}\left[\hat{\Theta}\,(s\mathbb{I} - \mathcal{L}_0)^{-1}\,\delta\hat{\rho}(0)\right]^*\end{pmatrix}, \tag{S14}$$

where

$$R(s) \equiv \begin{pmatrix}\mathcal{A}(s) & \mathcal{C}(s) \\ \mathcal{C}^*(s) & \mathcal{A}^*(s)\end{pmatrix} \tag{S15}$$

is related to the inverse response function of the cavity field. The crossover between stable and unstable behavior occurs when the susceptibility diverges. The susceptibility of the cavity field to the coherent scattering of photon by

the atoms is defined as the response function of the cavity at zero frequency [S10]. Accordingly, the crossover occurs when $\det[R(0)] = 0$. This happens when the following condition is met

$$\Delta_{\rm pc}^2(T) + \kappa^2 - 2\Delta_{\rm pc}(T)\mathrm{Im}[\mathcal{C}(0)] + 2\kappa\mathrm{Re}[\mathcal{C}(0)] = 0. \tag{S16}$$

Here $\mathcal{C}(0) \equiv \lim_{\epsilon\to 0^+}\mathcal{C}(-\mathrm{i}\omega + \epsilon)|_{\omega=0}$. In the above expression, the effective cavity shift reads

$$\Delta_{\rm pc}(T) \equiv \Delta_{\rm pc} - \frac{g_0^2 N}{\Delta_{\rm pa}}\langle \sin^2(k\hat{z})\rangle_{\rm th} = \Delta_{\rm pc} - \frac{g_0^2 N}{2\Delta_{\rm pa}}\left(1 - e^{-2\eta_T^2}\right). \tag{S17}$$

The second term on the right hand side of Eq. (S17) represents the frequency shift of the cavity due to thermal fluctuations of the atoms in the initial state $\hat{\rho}_{\rm th}$. Here, we defined the thermal Lamb-Dicke parameter as

$$\eta_T \equiv \eta\sqrt{\coth\left(\frac{\hbar\nu}{2k_B T}\right)}, \tag{S18}$$

where $\eta \equiv \sqrt{\nu_R/\nu}$ is the Lamb-Dicke parameter for an atom in the motional ground state and $\nu_R \equiv \hbar k^2/2M$ is the recoil frequency of the atom.

To evaluate the condition in Eq. (S16), we need to compute $\mathcal{C}(0)$, which corresponds to the susceptibility of the operator $\hat{\Theta}$. This is given by

$$\mathcal{C}(0) = \left(\frac{g_0\Omega N}{2\Delta_{\rm pa}}\right)^2 \lim_{\epsilon\to 0^+}\int_0^\infty \mathrm{d}t\, e^{-\epsilon t}\left\langle\left[\hat{\Theta}(t), \hat{\Theta}\right]\right\rangle_{\rm th}. \tag{S19}$$

For a tweezer trap frequency $\nu/2\pi \simeq 93\,\mathrm{kHz}$ and for an initial temperature $T \simeq 40\mu\mathrm{K}$, the Lamb-Dicke parameter $\eta_T \simeq 0.8$ is too large to make any perturbative approximation. We thus need to evaluate the response function of $\hat{\Theta}$ exactly. We first proceed to notice that $\hat{\rho}_{\rm th}$ is a product state where each atom is in a thermal state. Hence we can write

$$\left\langle\left[\hat{\Theta}(t), \hat{\Theta}\right]\right\rangle_{\rm th} = \frac{1}{N}\left\langle\left[\sin(k\hat{z}(t)), \sin(k\hat{z})\right]\right\rangle_{\rm th}, \tag{S20}$$

where $\hat{z}$ is the position operator of a generic single atom, and we dropped the index $j$ for convenience. Since $\hat{z}(t) = \hat{z}\cos(\nu t) + \hat{p}\sin(\nu t)/(M\nu)$, we use the Baker-Campbell-Hausdorff lemma to evaluate the commutator, finding

$$[\sin(k\hat{z}(t)), \sin(k\hat{z})] = -\mathrm{i}\sin(\nu t)\left\{\cos\left[k\hat{z} - k\hat{z}(t)\right] + \cos\left[k\hat{z} + k\hat{z}(t)\right]\right\}. \tag{S21}$$

The average over the thermal state of Eq. (S21) can be easily computed using the Wigner function representation of the thermal state. Putting everything together, we obtain

$$\begin{aligned}\mathcal{C}(0) =& -2\mathrm{i}e^{-\eta_T^2}\left(\frac{g_0\Omega}{2\Delta_{\rm pa}}\right)^2 N\lim_{\epsilon\to 0^+}\int_0^\infty \mathrm{d}t\, e^{-\epsilon t}\sin[\eta^2\sin(\nu t)]\cosh\left[\eta_T^2\cos(\nu t)\right]\\ \simeq& -2\mathrm{i}\eta^2 e^{-\eta_T^2}\left(\frac{g_0\Omega}{2\Delta_{\rm pa}}\right)^2 N\lim_{\epsilon\to 0^+}\int_0^\infty \mathrm{d}t\, e^{-\epsilon t}\sin(\nu t)\cosh\left[\eta_T^2\cos(\nu t)\right],\end{aligned} \tag{S22}$$

where information of the motional temperature appears through the Lamb-Dicke parameter $\eta_T$, and in going from the first to the second line we kept the leading order in $\eta^2$. The resulting integral in Eq. (S22) can be computed exactly by means of the identity

$$\cosh\left[\eta_T^2\cos(\nu t)\right] = I_0(\eta_T^2) + 2\sum_{n=1}^{\infty} I_{2n}(\eta_T^2)\cos(2n\nu t), \tag{S23}$$

where $I_n(x)$ is $n$-th order modified Bessel function of the first kind. We can compute $\mathcal{C}(0)$ by substituting Eq. (S23) into Eq. (S22) performing the integral and taking the limit $\epsilon \to 0^+$. Substituting this result into Eq. (S16) and solving for the pump strength we obtain the critical pump strength

$$\Omega_{\rm c} \equiv \sqrt{\frac{\nu\Delta_{\rm pa}^2(\Delta_{\rm pc}^2(T) + \kappa^2)}{\eta^2 g_0^2|\Delta_{\rm pc}(T)|N\varepsilon_{\rm 1D}(T)}}, \tag{S24}$$

where

$$\varepsilon_{1\mathrm{D}}(T) = e^{-\eta_T^2}\left[I_0(\eta_T^2) + 2\sum_{n=1}^{\infty}\frac{I_{2n}(\eta_T^2)}{1-4n^2}\right] \approx e^{-\eta_T^2}\frac{\sinh\eta_T^2}{\eta_T^2}. \tag{S25}$$

The last equality has not been formally derived. It has been obtained by expanding the modified Bessel functions up to high orders in $\eta_T$ and noticing the agreement with the Taylor expansion of the hyperbolic sine function.

We conclude this section with several remarks. First, the critical pump strength in Eq. (S24) includes both the effects of finite motional temperature of the atoms as well as the effects of non-linearities in the atomic motion resulting from the interaction with the cavity field in Eq. (S4). Had we neglected the non-linearities in the effective atomic potential, we would have obtained $\varepsilon_{1\mathrm{D}}(T) = 1$. The main consequence of the motional non-linearities is thus to shift the critical pump strength to higher values. Second, the effects of the temperature are two-fold. On the one hand, it shifts the cavity resonance through $\Delta_{\mathrm{pc}}(T)$. On the other hand, it leads the atoms to probe the non-linear potential through the thermal spread of the atomic wavefunction. Accordingly, when the temperature is sufficiently low, the dynamics can be approximated as linear. In this case, and to linear order in the displacement from equilibrium, only one collective mode is coupled to the cavity field. We call this mode the dominant mode [S11]. The critical pump strength can then be understood as the value at which the dominant mode becomes unstable. Finally, this insight leads to an alternative interpretation to the thermal effects and the role of non-linearities. The thermal shift in $\varepsilon_{1\mathrm{D}}(T)$ arises from the sum of two different contributions. One is the non-linear correction to the potential of the dominant mode that contributes with $\varepsilon_{1\mathrm{D}}(T)/N$. The other is the correction arising from the occupation of the other $N-1$ normal modes which couple to the dominant mode via the non-linearities. Each of these modes also contributes $\varepsilon_{1\mathrm{D}}(T)/N$ due to equipartition. The dominant mode thus couples to a bath of modes to which it can disperse energy. This results in an increase in the effective pump strength $\Omega_{\mathrm{c}}$ required to observe the crossover to self-organization.

### B. 2D Motion

We now generalize the result to the case of atoms moving both along and perpendicular to the cavity axis. The coupled mean field equation for the cavity and atomic motional state read

$$\begin{aligned}\dot{\hat{\rho}}_{\mathrm{at}} &= -\frac{\mathrm{i}}{\hbar}[\hat{H}_{2\mathrm{D}}, \hat{\rho}_{\mathrm{at}}] - \mathrm{i}\frac{\Omega g_0}{2\Delta_{\mathrm{pa}}}(\alpha+\alpha^*)\left[\sum_{j=1}^{N}\cos(k\hat{x}_j)\sin(k\hat{z}_j), \hat{\rho}_{\mathrm{at}}\right] - \mathrm{i}|\alpha|^2\frac{g_0^2}{\Delta_{\mathrm{pa}}}\left[\sum_{j=1}^{N}\sin^2(k\hat{z}), \hat{\rho}_{\mathrm{at}}\right],\\ \dot{\alpha} &= \left[\mathrm{i}\Big(\Delta_{\mathrm{pc}} - \frac{g_0^2}{\Delta_{\mathrm{pa}}}\sum_{j=1}^{N}\langle\sin^2(k\hat{z}_j)\rangle\Big) - \kappa\right]\alpha - \mathrm{i}\frac{g_0\Omega}{2\Delta_{\mathrm{pa}}}\left\langle\sum_{j=1}^{N}\cos(k\hat{x}_j)\sin(k\hat{z}_j)\right\rangle,\end{aligned} \tag{S26}$$

where

$$\hat{H}_{2\mathrm{D}} \equiv \sum_j\left\{\frac{\hat{\mathbf{p}}_j^2}{2M} + \frac{M\nu^2}{2}[(\hat{z}_j - z_{0j})^2 + \hat{x}_j^2] - \frac{\hbar\Omega^2}{4\Delta_{\mathrm{pa}}}\cos^2(k\hat{x}_j)\right\}, \tag{S27}$$

and $\hat{\mathbf{p}}_j = (\hat{p}_{xj}, \hat{p}_{zj})$. Proceeding in the same way as for the 1D case, we obtain the same condition of Eq. (S16) for the poles of the cavity susceptibility, but with $\mathcal{C}(s)$ substituted by

$$\mathcal{C}_{2\mathrm{D}}(s) = \left(\frac{g_0\Omega}{2\Delta_{\mathrm{pa}}}\right)^2 N\lim_{\epsilon\to0^+}\int_0^\infty \mathrm{d}t\, e^{-\epsilon t}\left\langle[\cos(k\hat{x}(t))\sin(k\hat{z}(t)), \cos(k\hat{x})\sin(k\hat{z})]\right\rangle_{\mathrm{th}}. \tag{S28}$$

Since the initial thermal state is factorized, we have written Eq. (S28) in terms of the average over a single atom. In this case, the evolution of $\hat{x}(t)$ is governed by the harmonic potential of the tweezer and the $\cos^2(k\hat{x})$ potential corrections introduced by the standing wave of the side pump, as shown in Eq. (S27) . If we approximate the cosine potential as $\cos^2(k\hat{x}) \simeq 1-(k\hat{x})^2$, we obtain the leading correction to the trap frequency along the $x$-axis as a function of the pump strength. In this case, it is possible to obtain a closed expression for Equation (S28) by following the same steps and approximations we illustrated for the case of motion along a single direction. However, the resulting expression for the critical pump strength is given in terms of an implicit function of $\Omega$ whose zeros correspond to $\Omega_c$. The difficulty of obtaining an explicit expression for $\Omega_c$ follows from the fact that the Lamb-Dicke parameters and trap frequency for the motion along the $x$-axis depend on $\Omega$. To obtain a close expression for $\Omega_c$, we thus neglect the shift induced by the pump on the trap frequency along the $x$-axis. While this approximation seems *a priori* not justified, we

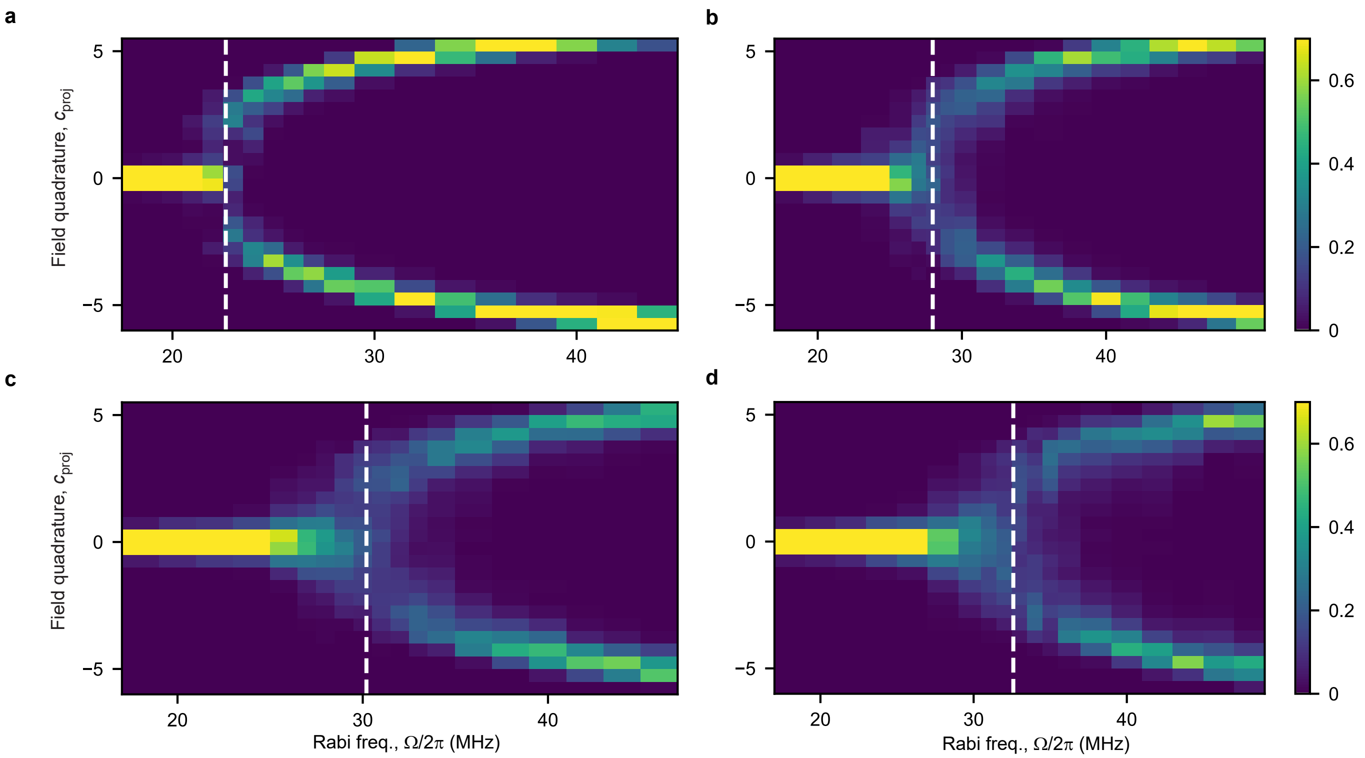


Figure S1. Numerical results of the bifurcation diagram for the field projection as computed from Eqs. (S30a-S30g) for different motional temperatures: **a,** $T = 20\,\mu$K, **b,** $T = 41\,\mu$K, **c,** $T = 50\,\mu$K and **d,** $T = 60\,\mu$K. The white dashed vertical line corresponds to the analytical prediction from the 2D model. The parameters $N = 20$, $\Delta_{\text{pa}} = -2\pi \times 80\,\text{MHz}$, and $\Delta_{\text{pc}} = -2\pi \times 1.9\,\text{MHz}$ are the same for all subplots. The color bar shows the probability density.

check that the final result agrees with the numerical simulations where this effect is included [see Sec. III]. Neglecting this Ω-dependent shift, one obtains the same expression for the critical pump strength as in 1D, i.e., Eq. (S24), but where now $\varepsilon_{1\text{D}}(T)$ is substituted by

$$\varepsilon(T) \equiv e^{-2\eta_T^2}\left[I_0(2\eta_T^2) + 2\sum_{n=1}^{\infty}\frac{I_{2n}(2\eta_T^2)}{1-4n^2}\right] \approx e^{-2\eta_T^2}\,\frac{\sinh[2\eta_T^2]}{2\eta_T^2}. \tag{S29}$$

Within these approximations, the only modification induced by the additional motional direction is to double the contribution of the thermal Lamb-Dicke parameter.

## III. NUMERICAL SIMULATION OF THE MEAN-FIELD SEMICLASSICAL DYNAMICS

We also compute the bifurcation diagram for the cavity field output by solving the semiclassical equations for the evolution of the expectation value of the system's degrees of freedom in Eq. (S1). Specifically, we numerically solve

the following set of equations

$$\partial_t \sigma_n^z = -2\gamma\left(1+\sigma_j^z\right) + \mathrm{i}\Omega(x)\left(\sigma_j^- - \sigma_j^+\right) + 2\mathrm{i}g_0\sin(kz_j)\left(\sigma_j^- c^* - \sigma_j^+ c\right), \tag{S30a}$$

$$\partial_t \sigma_n^- = \Delta_A \sigma_j^- + \mathrm{i}\left[\frac{\Omega(x)}{2} + g_0\sin(kz_j)c\right]\sigma_j^z, \tag{S30b}$$

$$\partial_t c = \Delta_C c - \mathrm{i}g_0\sum_{j=1}^{N}\sin(kz_j)\sigma_j^-, \tag{S30c}$$

$$\partial_t p_{zj} = -M\nu^2 z_j - \hbar k g_0\cos(kz_j)\left(c^*\sigma_j^- + c\sigma_j^+\right), \tag{S30d}$$

$$\partial_t p_{xj} = -M\nu^2 x_j - \frac{1}{2}\partial_x\Omega(x)\left(\hat\sigma_j^+ + \hat\sigma_j^-\right), \tag{S30e}$$

$$\partial_t z_j = \frac{p_{zj}}{M}, \tag{S30f}$$

$$\partial_t x_j = \frac{p_{xj}}{M}, \tag{S30g}$$

where for a generic system operator $\hat a$ we defined $a \equiv \langle \hat a\rangle$. The effect of temperature enters into the mean field dynamics by sampling the initial position and momentum from a thermal distribution at temperature $T$. We consider the cavity to be initially in vacuum $c(0)=0$ and the atoms to be in their ground state $\hat\sigma_j^z(0)=-1$ and $\hat\sigma_j^+(0)=0$.

We compute the field projection following the same procedure described for the experiment. In Fig. S1, we compare the results of the numerical simulations for the field projection as a function of the pump strength $\Omega$ with the prediction of the critical pump strength derived in Sec. II from a 2D model. We find good agreement between the two methods. The numerical simulation accounts for the internal dynamics of the atoms and for atomic saturation, while the analytical results in Sec. II are obtained under the assumption of linear response and adiabaticity of the atomic internal dynamics. The agreement between the analytical prediction and the numerical simulation is thus an *a posteriori* confirmation that our approximated model correctly captures the critical point for atomic self organization.

## IV. THEORETICAL CALCULATION OF OPTOMECHANICAL SUSCEPTIBILITY

We first present an approximate analytical expression for the susceptibility $\chi$ where we approximate the potential energy of the dominant mode as only containing terms up to fourth order in $z_{\mathrm{dom}}$, following Landau's prescription. From now on, we drop the "dom" subscript for convenience of notation. The thermally averaged displacement of the dominant mode is given by

$$\langle z\rangle_{\mathrm{approx}} = \frac{\int_{-\infty}^{+\infty} z\exp\Big(-\frac{N}{\sigma^2}\big(\frac{\Omega^2}{6\Omega_{\mathrm{c}}{}^2}(k^2z^2-3)z^2 + \frac{1}{2}(z-\delta z)^2\big)\Big)dz}{\int_{-\infty}^{+\infty}\exp\Big(-\frac{N}{\sigma^2}\big(\frac{\Omega^2}{6\Omega_{\mathrm{c}}{}^2}(k^2z^2-3)z^2 + \frac{1}{2}(z-\delta z)^2\big)\Big)dz}. \tag{S31}$$

Here we have defined $\sigma = \sqrt{\frac{k_B T}{M\nu^2}}$, which gives the standard deviation of the atomic thermal density distribution in a harmonic tweezer. From this, we obtain an approximation for $\chi$:

$$\chi_{\mathrm{approx}} \simeq \frac{\partial\langle z\rangle_{\mathrm{approx}}}{\partial(\delta z)}\bigg|_{\delta z=0} = \frac{\int_{-\infty}^{+\infty}\frac{Nz^2}{\sigma^2}\exp\Big(-\frac{N}{\sigma^2}\big(\frac{\Omega^2}{6\Omega_{\mathrm{c}}{}^2}(k^2z^2-3)z^2+\frac{1}{2}z^2\big)\Big)dz}{\int_{-\infty}^{+\infty}\exp\Big(-\frac{N}{\sigma^2}\big(\frac{\Omega^2}{6\Omega_{\mathrm{c}}{}^2}(k^2z^2-3)z^2+\frac{1}{2}z^2\big)\Big)dz}$$
$$= \frac{\pi(3N(r^2-1)I_{-\frac{1}{4}}(\frac{3N(r^2-1)^2}{16k^2r^2\sigma^2}) - (3N(r^2-1)^2+8k^2r^2\sigma^2)I_{\frac{1}{4}}(\frac{3N(r^2-1)^2}{16k^2r^2\sigma^2}) + 3N(r^2-1)^2(I_{\frac{3}{4}}(\frac{3N(r^2-1)^2}{16k^2r^2\sigma^2}) - I_{\frac{5}{4}}(\frac{3N(r^2-1)^2}{16k^2r^2\sigma^2})))}{4\sqrt{2}k^2r^2(r^2-1)\sigma^2K_{\frac{1}{4}}(\frac{3N(r^2-1)^2}{16k^2r^2\sigma^2})}, \tag{S32}$$

where $r \equiv \Omega/\Omega_{\mathrm{c}}$ and $I_\alpha(x)$ and $K_\alpha(x)$ are modified Bessel functions of the first and second kind respectively.

We can similarly obtain an integral expression for $\chi$ where we keep the sinusoidal form of the cavity potential. In this case, the average dominant mode displacement is

$$\langle z\rangle = \frac{\int_{-\infty}^{+\infty} z\exp\Big(-\frac{N}{4k^2\sigma^2}\big(-r^2+2k^2(z-\delta z)^2+r^2\cos(2kz)\big)\Big)dz}{\int_{-\infty}^{+\infty}\exp\Big(-\frac{N}{4k^2\sigma^2}\big(-r^2+2k^2(z-\delta z)^2+r^2\cos(2kz)\big)\Big)dz}. \tag{S33}$$

Thus, the expression for $\chi$ becomes

$$\chi \simeq \frac{\partial\langle z\rangle}{\partial(\delta z)}\bigg|_{\delta z=0} = \frac{\int_{-\infty}^{+\infty} \frac{Nz^2}{\sigma^2} \exp\Big(-\frac{N}{4k^2\sigma^2}\big(-r^2+2k^2z^2+r^2\cos(2kz)\big)\Big)dz}{\int_{-\infty}^{+\infty} \exp\Big(-\frac{N}{4k^2\sigma^2}\big(-r^2+2k^2z^2+r^2\cos(2kz)\big)\Big)dz}. \tag{S34}$$

By numerically computing the integrals in Eq. (S34), we obtain the theory curves shown in Fig. 4c of the main text.

---


[S1] M. Aspelmeyer, T. J. Kippenberg, and F. Marquardt, Cavity optomechanics, Rev. Mod. Phys. **86**, 1391 (2014).

[S2] V. Vuletić and S. Chu, Laser cooling of atoms, ions, or molecules by coherent scattering, Phys. Rev. Lett. **84**, 3787 (2000).

[S3] V. Vuletić, H. W. Chan, and A. T. Black, Three-dimensional cavity doppler cooling and cavity sideband cooling by coherent scattering, Phys. Rev. A **64**, 033405 (2001).

[S4] P. Domokos and H. Ritsch, Mechanical effects of light in optical resonators, J. Opt. Soc. Am. B **20**, 1098 (2003).

[S5] P. Domokos and H. Ritsch, Collective cooling and self-organization of atoms in a cavity, Phys. Rev. Lett. **89**, 253003 (2002).

[S6] J. K. Asbóth, P. Domokos, H. Ritsch, and A. Vukics, Self-organization of atoms in a cavity field: Threshold, bistability, and scaling laws, Phys. Rev. A **72**, 053417 (2005).

[S7] S. Schütz, S. B. Jäger, and G. Morigi, Thermodynamics and dynamics of atomic self-organization in an optical cavity, Phys. Rev. A **92**, 063808 (2015).

[S8] S. B. Jäger, S. Schütz, and G. Morigi, Mean-field theory of atomic self-organization in optical cavities, Phys. Rev. A **94**, 023807 (2016).

[S9] M. Nairn, L. Giannelli, G. Morigi, S. Slama, B. Olmos, and S. B. Jäger, Spin-self-organization in an optical cavity facilitated by inhomogeneous broadening (2024), arXiv:2407.19706 [cond-mat.quant-gas].

[S10] M. Le Bellac, F. Mortessagne, and G. G. Batrouni, *Equilibrium and Non-Equilibrium Statistical Thermodynamics* (Cambridge University Press, 2004).

[S11] When the interatomic separation is an integer (half-integer) multiple of $\lambda$ the dominant mode is the center-of-mass (antiphase) mode where neighboring atoms move in phase (in phase opposition).
